# Supplementary material for: User-aware WLAN Transmit Power Control in the Wild
Source: arXiv:2302.10676 source file (2023-02-21)
Supplement: Supplementary file 1 [file 9_appendix.tex]

\appendix

\section{Utility function}
Eventually more details here.

\section{Comparison of reference point selection strategies}
We here compare the reference point selection strategies on both simulator (Fig.~\ref{fig:select:compare:sim}) and real network(Fig.~\ref{fig:select:compare}). 
 and Fig.~\ref{} show the distribution of utilities. 
\begin{figure*}[t!]
    \subfigure[All points]
    {
        \includegraphics[width=0.99\columnwidth]{figures/RPS_cluster_random_reward_CDF_all.pdf}  
        \label{fig:}
    }
    \subfigure[Isolated points]{%
        \includegraphics[width=0.99\columnwidth]{figures/RPS_cluster_random_reward_CDF_isolated_small.pdf}
        \label{fig:}
    }    
    \caption{Simulator-based. Utility distributions over all 1.8M points and 5.8K isolated points}
  \label{fig:select:compare:sim}
\end{figure*}

\begin{figure*}[t!]
    \subfigure[Interference]
    {
        \includegraphics[width=0.99\columnwidth]{figures/evaluation/STA/Interference_reduced_CDF_STA_select222.pdf}  
        \label{fig:}
    }
    \subfigure[Bad coverage]{%
        \includegraphics[width=0.99\columnwidth]{figures/evaluation/STA/DownlinkRSSIdBm_reduced_CDF_STA_select_random_vs_cluster_log_bad_222.pdf}
        \label{fig:}
    }    
    \caption{Deployment-based. }
  \label{fig:select:compare}
\end{figure*}

\section{Evaluation of simulator assumptions}

\begin{figure*}[t!]
    \subfigure[Pearson R]
    {
        \includegraphics[width=0.99\columnwidth]{figures/evaluation/AP/pearson_CDF.pdf}  
        \label{fig:}
    }
    \subfigure[p-value]{%
        \includegraphics[width=0.99\columnwidth]{figures/evaluation/AP/pvalues_CDF.pdf}
        \label{fig:}
    }    
    \caption{Correlation between estimated and real interferences through pearson R correlations between interference distributions over APs. (all experiments)}
  \label{fig:wfh}
\end{figure*}

\section{Evaluation of imputation}

\begin{figure}
    \subfigure[All points]
    {
        \includegraphics[width=0.47\textwidth]{figures/AE_Guess_from_N_N71F_16_2.pdf}  
        \label{fig:}
    }
    \subfigure[Isolated points]{%
        \includegraphics[width=0.47\textwidth]{figures/AE_Guess_from_N_16_2.pdf}
        \label{fig:}
    }    
    \caption{Performance depending on number of available neighbors}
  \label{fig:wfh}
\end{figure}

\begin{figure}
    \includegraphics[width=\columnwidth]{figures/mean_absolute_error_ml_train_test_naive_N71F.pdf}
    \caption{Per-AP model performance on train and test datasets}
    \label{fig:c}
\end{figure}

\section{Deployment evaluation}
Here we put more thorough evaluation of real network experiments.

\subsection{Impact on tx rate}
\begin{figure}
    \includegraphics[width=\columnwidth]{figures/evaluation/STA/Txrate_Mbps_fullpow_lim_CDF_STA.pdf}
    \caption{Transmission rate.}
    \label{fig:tx:rate}
\end{figure}

% \begin{figure*}
%     \subfigure[Transmit vs. Receive rates]{%
%         \includegraphics[width=.99\columnwidth]{figures/evaluation/STA/global_comparison_sta_txrx.pdf}  
%         \label{fig:sta:txrxrate}
%     }
%     \subfigure[Downlink vs. Uplink signal quality]{%
%         \includegraphics[width=.99\columnwidth]{figures/evaluation/STA/global_comparison_sta_dlul.pdf}  
%         \label{fig:sta:rxrate}
%     }
%     \caption{\textbf{Comparison of uplink and downlink}}
%   \label{fig:downup}
% \end{figure*}
